# Supplementary material for: Dynamic Joint Communications and Sensing Precoding Design: A Lyapunov Approach
Source: arXiv:2503.14054 source file (2025-03-18)
Supplement: Supplementary file 1 [file Appendix.tex]

\appendix %[Proof of Proposition \ref{Prop_ComMDP}]
\subsection{Proof of Proposition \ref{Prop_ComMDP}}
\label{App_ComMDP}
% First, we show the former via a counterexample. 
% Specifically, we show the
% the following deterministic policy induces a Markov chain with two recurrent classes, contradicting the unichain structure.
% %Without loss of generality, suppose the battery capacity $E=5$.
% The policy works as follows: it takes a new sample and transmits it whenever the energy level $e(t)$ is $3$; otherwise, it chooses the idle action. 
% In the induced Markov chain, the set of states ${ \{ (e,\theta,\varphi)\}_{\{e\le 3,\, \theta=1,2,\dots,N, \varphi\ge \theta\} } },$ and 
% ${ \{ (E,N, N)\} },$
% are two different recurrent classes, and 
% the set of states ${ \{ (e,\theta,\varphi)\}_{\{e > 3,\, \theta\neq N, \varphi\ge \theta\}} },$ are transient states. Thus, the Markov chain has more than one recurrent class, which completes the first part of proof.
%The induced Markov chain for the $e(t)$ is shown in Fig. \ref{Fig_CEx}, which is multichain.
To show the MDP is communicating, it is sufficient to find a randomized policy that induces a recurrent Markov chain, i.e., 
a policy  under which  any state of the arbitrary pair of states ${s=(e,\theta,\varphi)}$ and ${ s'=(e',\theta',\varphi')}$ in $\mathcal{S}$ is accessible from the other one \cite[Proposition 8.3.1]{Puterman_Book}.
% every pair of states ${s=(e,\theta,\varphi)}$ and ${ s'=(e',\theta',\varphi')}$ in $\mathcal{S}$ is accessible from each other \cite[Proposition 8.3.1]{Puterman_Book}.
 To have a shorthand notation, let's define $c\triangleq \ct + \cs$. 
We define the following policy: the policy takes the idle action $a =0$ with probability $1$ at any state where
${ e < c }$,
%$(e(t) < c^{\mathrm{s}} + c^{\mathrm{t}}, \theta(t))$, 
and in all the other states,  randomizes between the idle action $a=0$ and the sample and transmit action $a=2$ with probability $0.5$.
We consider two cases: $e' \ge e$ and $e' < e$. 
For the case where $e' \ge e$, realizing action $a = 0$ for at least ${ x \triangleq e' - e + 2c } $ consecutive slots, starting from $(e,\theta,\varphi)$, leads to state 
${(e' + 2c, 
\theta +x,
\varphi +x,
) }$ with a positive probability (w.p.p.);
then taking action $a = 2$ leads to state $(e'+c, 1, 1)$ w.p.p., recall that action $a = 2$ requires $c= \ct + \cs$ units of energy. 
Subsequently, taking action $a = 0$ for $\varphi'-\theta'$ consecutive
slots followed by action $a=2$ 
leads to state $(e',1, \varphi'-\theta'+1)$ w.p.p.. Now,    taking action $a = 0$ for ${\theta'-1 } $ consecutive slots leads to state $ (e',\theta', \varphi') $ w.p.p..

For the case where $e' < e$, supposing $e\ge c$ without loss of generality,  taking action $a = 2$ for ${ \floor{\frac{e }{c  } } } $ consecutive slots leads 
  to state $(r, 1,1)$, where $r\triangleq e-c\floor{\frac{e }{c }}$, w.p.p.. Then taking  action $a = 0$ for  $c-r$ slots leads to state $(c, 1+c-r, 1+c-r)$ w.p.p., and, subsequently, taking action $a=2$ 
  leads to state $(0, 1, 1)$ w.p.p..
  Now, following the same procedure for the case $e'\ge e$, described above,   leads to state $(e',\theta',\varphi') $ w.p.p., which completes the proof. 
%-----------

\subsection{Proof of Proposition  \ref{Prop_dis_blf_age}}\label{App_dist_blf}
 As the source is Markov, the necessary information required for calculating the belief from the complete information $I_{\mathrm{C}}(t)$ are: the last state of the source sampled, i.e., $\tx$, and how long ago that sample has been taken which is the age of that sample, i.e., the AoI at the transmitter. Thus, we have 
    \begin{equation}
        \begin{array}{cc}
             b(t) = \Pr\{X(t)=1\,\big|\,I_{\mathrm{C}}(t)\}=\Pr\{X(t)=1\,\big|\,\theta(t), \tx\}= \Pr\{X(t)=1\,\big|\,X(t-\theta(t)) = \tx\},
        \end{array}
    \end{equation}
    which equals to the $\theta(t)-$step transition probability of the (source) Markov chain. For the Markov chain, it follows that (see, e.g., \cite{Kam_Towards_eff_2018})
    $\Pr\{X(t)=1\,\big|\,X(t-\theta(t)) = 1\}= 0.5\left(1+(2p-1)^{\theta(t)} \right)$, and 
    $\Pr\{X(t)=1\,\big|\,X(t-\theta(t)) = 0\}= 1- 0.5\left(1+(2p-1)^{\theta(t)} \right)$, which completes proof.

%-------------------
    \subsection{Proof of Proposition \ref{Prop_AoII_blf_gnr}}\label{App_AoII_blf_gnr}
     Generally the belief update depends on the dynamic of $X(t)$ and $\hx$.
 The dynamic of $X(t)$ is independent from action and observation.
 Let's denote $\mathcal{B}\triangleq \{b_i(t)\}_{i= 0,1,\ldots}$.
Given an action and observation, there are different possibilities for $b(t+1)$.
We first consider the case where $a(t)=0$, implying that $\hat{X}(t+1)=\hx$. Let's start off to obtain $b_0(t+1)$ below:
\begin{equation}
    \begin{array}{ll}
        & b_0(t+1)  
        \triangleq \Pr\{\delta(t+1)=0\,\big|\, a(t)=0,\mathcal{B},o(t+1)\} = 
    \Pr\{\delta(t+1)=0\,\big|\, a(t)=0,\mathcal{B}\} 
    \\ & 
   \stackrel{(a)}
    {=} \Pr\{X(t+1)=X(t)\}\Pr\{\hat{X}(t+1)= X(t) \,\big|\, a(t)=0,\mathcal{B}\} 
    \\&
    +
    \Pr\{X(t+1)=1-X(t)\}\Pr\{\hat{X}(t+1)= 1-X(t)\,\big|\, a(t)=0,\mathcal{B}\}
    \\&
    \stackrel{ (b)} {=}
    pb_0(t) + (1-p) (1-b_0(t) ),
    \end{array}
\end{equation}
where $(a)$ follows from the independence of the source process and the estimate,
and $(b)$ follows from the facts that $\Pr\{X(t+1)=X(t)\}=p$, 
$\Pr\{\hat{X}(t+1)= X(t) \,\big|\, a(t)=0,\mathcal{B}\}=\Pr\{\hat{X}(t)= X(t) \,\big|\,\mathcal{B}\}=\Pr\{\delta(t)=0\,\big|\,\mathcal{B}\}=b_0(t)$, and 
$\Pr\{\hat{X}(t+1)= 1-X(t)\,\big|\, a(t)=0,\mathcal{B}\}=
\Pr\{\hat{X}(t)= 1-X(t) \,\big|\,\mathcal{B}\}=\Pr\{\delta(t)\neq 0\,\big|\,\mathcal{B}\}=1-b_0(t).
$
For the other beliefs, i.e., $b_i(t+1),\,i=1,\dots$, we should calculate the probability of ${X(t+1) \neq \hat{X}(t+1)}$ given the facts that the AoII can increase only by one and $\hat{X}(t+1)=\hx$. We have 
\begin{equation}\label{Eq_blf_proof_a0}
    \begin{array}{ll}
         b_1(t+1)  
        & =\Pr\{\delta(t)=0, X(t+1) \neq \hat{X}(t+1)\,\big|\, a(t)=0,\mathcal{B}\} 
       \\&
         \stackrel{(a)}
         {= }
    \Pr\{\delta(t)=0\,\big|\, \mathcal{B}\} 
    \Pr\{X(t+1) = 1-X(t)\} = 
    b_0(t) (1-p),
    \end{array}
\end{equation}
where $(a)$ follows from  the condition probability rule that $\Pr\{A,B\}=\Pr\{A\,\big|\,B\}\Pr\{B\}, $
and $\Pr\{X(t+1)\neq \hat{X}(t+1)\,\big|\,\delta(t)=0\}= \Pr\{X(t+1) = 1-X(t)\}.$
Similarly, for $i=2,\dots$, we have
\begin{equation}
    \begin{array}{ll}
         b_i(t+1)  
        & =\Pr\{\delta(t)=i-1, X(t+1) \neq \hat{X}(t+1)\,\big|\, a(t)=0,\mathcal{B}\} 
       \\&
         \stackrel{(a)}
         {= }
    \Pr\{\delta(t)=i\,\big|\, \mathcal{B}\} 
    \Pr\{X(t+1) = X(t)\} = 
    b_i(t) p,
    \end{array}
\end{equation}
where $(a)$ follows from the same fact used in \eqref{Eq_blf_proof_a0} but
$\Pr\{X(t+1)\neq \hat{X}(t+1)\,\big|\,\delta(t)\neq 0\}= \Pr\{X(t+1) = X(t)\}$, using the fact that $\delta(t)\neq 0$ means $X(t)\neq\hx$.  % . We remind that $\hat{X}(t+1)=\hx$, as it is supposed that $a(t)=0$.

Now we consider the case where $a(t) =1$. This implies that $\hat{X}(t+1)$ could be $1-\hat{X}(t)$. 
However,  $\rho(t+1)=1$ implies that the transmission was not successful and thus $\hat{X}(t+1)=\hx$. Therefore, the belief update when $a(t)=1$ and $\rho(t+1)=1$ is equivalent to the belief update for $a(t)=0$, which is given above. Suppose $a(t)=1$ and $\rho(t+1)=0$, which implies $\hat{X}(t+1) = 1-\hx$ since $a(t)=1$ means $\hat{X}(t)\neq \tx$. 
The belief update when $a(t)=1$ and $\rho(t+1)=0$ follows the similar way of that for $a(t) = 0$ by replacing $\hat{X}(t+1)= 1- \hat{X}(t)$. 
%except that the source should flip in order to have  $\Pr\{X(t+1)\neq \hat{X}(t+1)$

Finally, consider the case where $a(t)=2$, which means that $X(t)$ is observed at slot $t$ and $\tilde{X}(t+1) = X(t)$. Again we need to consider whether $\hat{X}(t+1)$ equals $\hx$ or nor, which can be determined by $\rho(t+1)$. There are two different cases:  1) $\rho(t+1)=1$, which means ${\hat{X}(t+1)\neq \tilde{X}(t+1)}$, and since $\tilde{X}(t+1)=X(t)$, we have $\hat{X}(t+1) \neq X(t)$; and 
2) $\rho(t+1)=0$, which means $\hat{X}(t+1)={X}(t)$. Accordingly, the belief update for $a(t)=2$ and  $\rho(t+1)=1$ can be obtained by
\begin{equation}\nonumber
    \begin{array}{ll}
        & b_0(t+1)  = \Pr\{X(t+1)=\hat{X}(t+1)\,\big|\,\hat{X}(t+1)\neq X(t),\,\mathcal{B}\}
         =\Pr\{X(t+1)\neq {X}(t)\} = 1-p, 
    \\ & 
    b_i(t+1) = \Pr\{\delta(t)=i-1, X(t+1) \neq \hat{X}(t+1)\,\big|\, \hat{X}(t+1)\neq X(t),\,\mathcal{B}\}
    \\&
    =
    \Pr\{\delta(t)=i-1\,\big|\,\mathcal{B}\}
    \Pr\{{X}(t+1) =  X(t)\} = b_{i-1}(t)p.
    \end{array}
\end{equation}
For  $a(t)=2$ and  $\rho(t+1)=0$, the AoII can be $0$, or $1$, with the following probabilities:
\begin{equation}\nonumber
    \begin{array}{ll}
        & b_0(t+1)  = \Pr\left\{X(t+1)=\hat{X}(t+1)\,\big|\,\hat{X}(t+1)= X(t),\,\mathcal{B}\right\}
         =\Pr\{X(t+1) =  {X}(t)\} = p, 
    \\ & 
    b_1(t+1) = \Pr\left\{X(t+1)\neq \hat{X}(t+1)\,\big|\,\hat{X}(t+1)= X(t),\,\mathcal{B} \right\}
    =\Pr\left\{X(t+1) \neq {X}(t)\right\} = 1-p, 
    \end{array}
\end{equation}
which completes the proof. 

%--------------------------
\subsection{Proof of Proposition \ref{Prop_AoII_blf_prfch}}\label{App_AoII_blf_prfch}
The key idea of the proof is that whenever the sampling and transmission action $a(t)=2$ is being taken, the belief update becomes  independent of the current belief, as it is suggested by \eqref{Eq_BlfupAoII_reset}. 
When  $a(t)=0$, the belief evolves by a specific pattern given by \eqref{Eq_BlfupdAoII_idle}. 
Thus, to compute the belief at slot $t$, the only required information is that  how  many slots ago the last sampling was performed, or, in other words, how many consecutive slots the belief  update follows \eqref{Eq_BlfupdAoII_idle}. This information is the AoI at the transmitter $\theta(t)$. To easily describe the belief update next, the AoII evolution, as a controlled Markov chain, is shown in Fig. \ref{Fig_AoII_evl}, where  
%--------------------------  Markov chain of the AoII -----
$v(t)$ is given by 
 \begin{equation}\label{Eq_vt}
     \begin{array}{cc}
 v(t) \triangleq
\left\{\begin{array}{ll}
 1-p, & \text{if}~~   a(t) = 0,
   \\
p , & \text{if}~~   a(t) = 2.
 \end{array}\right. 
    \end{array}
 \end{equation}  
\begin{figure}[t!]
    \centering
    \includegraphics[width=.5\textwidth]{Figures/AoII_blf_MC}    
    \caption{The evolution of the AoII under  the perfect channel, where $v(t)$ is given by \eqref{Eq_vt}.
    }
    \label{Fig_AoII_evl}
\end{figure}
%-------------

Provided that $\theta(t)$ is given, we calculate the belief below starting with $b_0(t)$:
\begin{equation}
 \begin{array}{ll}
   b_0(t) = \Pr\left\{ X(t) = \hat{X}(t)\,\big|\,\theta(t) \right\} 
    \stackrel{(a)}
    {=}
   \Pr\left\{ X(t) = \hat{X}(t)\,\big|\,\hx=X(t-\theta(t)) \right\} 
    \stackrel{(b)}
    {=}
   0.5(1+(2p-1)^{\theta(t)}),
 \end{array}
\end{equation}
where $(a)$ follows from the fact that the estimate is the last received sample, and $(b)$ follows from the $K$-step transition probability of the Markov chain, where $K=\theta(t)$.
For ${b_i(t),i=1,\dots}$, first, the AoII cannot be larger than $\theta(t)$; thus, $b_i(t)=0,\,\forall \, i > \theta(t)$. 
Moreover, to have ${ \delta(t) = i,\,i=1,\dots,\theta(t) }$: i) the AoII at time $t-i$ must be zero and 2) the AoII must not reset to $0$ between  slots $t-i$ and  $t$ (i.e., for $i$ consecutive slots). 
The probability of occurrence of event (i)  is $\Pr\{\delta(t')=0\,\big|\,\theta(t')=\theta(t)-i\} = 0.5(1+(2p-1)^{\left(\theta(t)-i\right)})$, and, 
it follows from Fig. \ref{Fig_AoII_evl}  that the probability of occurrence of event (ii) is $(1-p)(1-v(t))^{(t-i-t-1)}$, where $v(t)=1-p$ since $a(t)=0$.
Multiplying these two completes the proof.
% This is, for every $i=1,\dots,\theta(t)$,
% \begin{equation}
%  \begin{array}{ll}
%    b_i(t) = \Pr\left\{ \delta(t-i)=0,\delta(t-i+1)\neq 0,\dots, \delta(t)\neq 0\,\big|\,\theta(t) \right\} 
%     \stackrel{(a)}
%     {=}
%    \Pr\left\{ X(t) = \hat{X}(t)\,\big|\,\hx=X(t-\theta(t)) \right\} 
%     \stackrel{(b)}
%     {=}
%    0.5(1+(2p-1)^{\theta(t)}),
%  \end{array}
% \end{equation}
